# Supplementary material for: Light yield and radiation hardness studies of scintillator strips with a filler
Source: arXiv:1711.11393 source file (2018-08-06)
Supplement: Supplementary file 1 [file AppendixEng.tex]

\begin{table}[htb]
  \begin{center}
		\begin{tabular}{|c|c|c|}
			\hline
			Scintillator & T20 & t50 \\
				& 20\% transmittance & mechanical \\
				&	& strength \\
			\hline
			SCSN-81 & 10 & 6.2  \\
			\hline
			BC - 408 & 6 & 5.1 \\
			\hline
			UPS-98RH & 8 & 5.8 \\
			\hline
			UPS-923A & 10 & 8.2\\
			\hline
		\end{tabular}
  \end{center}
  \caption{Long-term stability of light yield and mechanical strength \cite{Grinev} }
	\label{table: Act2003}
\end{table}

\begin{table}[htb]
  \begin{center}
		\begin{tabular}{|c|c|c|c|}
			\hline
			Sample & before & after 0.5 Mrad & 1 .0 Mrad \\
			\cline{3-4}	
			scintillator	& Light yield &\multicolumn{2}{c|}{Relative decrease } \\
				&  ($N_{p.e.}$) &\multicolumn{2}{c|}{in light yield [\%]} \\
			\hline
				SCSN81 & $9.14 \pm 0.14$ & $2.2 \pm 0.1$ & $8.0 \pm 0.2$\\
			\hline
				SCSN38D & $10.46 \pm 0.14$ & $5.6 \pm 0.1$ & $13.6 \pm 0.3$ \\
			\hline
				BC408 & $8.94 \pm 0.13$ & $8.1 \pm 0.2$ & $14.6 \pm 0.4$ \\
			\hline
		\end{tabular}
  \end{center}
  \caption{\small Light yield of scintillator vs dose \cite{CDFRUN1EMtile}}
	\label{table: tile95}
\end{table}
